# Supplementary material for: Searching for a source without gradients: how good is infotaxis and how to beat it
Source: arXiv:2112.10861 ancillary file (2022-06-15)
Supplement: Supplementary file 1 [file SM_additional_information.pdf]

Supplementary Material for

# Searching for a source without gradients: how good is infotaxis and how to beat it


Aurore Loisy and Christophe Eloy

*Aix Marseille Univ, CNRS, Centrale Marseille, IRPHE, Marseille, France*


Contents


- Section 1: Propagation-detection model in $n$ dimensions
- Section 2: Additional information on our methodology
- Section 3: Naive policies
- Section 4: Explicit calculation of the expected entropy
- Section 5: Additional results on infotaxis
- Section 6: N-step infotaxis algorithm
- Section 7: Additional results on space-aware infotaxis
- Section 8: Additional information on deep reinforcement learning
- Section 9: List of other materials

# 1 Propagation-detection model in $n$ dimensions

## 1.1 Model of propagation

We first derive the expression of the mean concentration of odor particles due to a point source. A source located at $\boldsymbol{x}^s$ emits detectable particles at rate $R$ with finite lifetime $\tau$, which disperse in an isotropic medium characterized by an effective diffusivity $D$. The mean stationary concentration field $c(\boldsymbol{x}^a|\boldsymbol{x}^s)$ satisfies

$$D\nabla^2 c(\boldsymbol{x}^a|\boldsymbol{x}^s) - \frac{1}{\tau}c(\boldsymbol{x}^a|\boldsymbol{x}^s) + R\delta(\boldsymbol{x}^a - \boldsymbol{x}^s) = 0. \tag{S1}$$

The solution is

$$c(\boldsymbol{x}^a|\boldsymbol{x}^s) = -\frac{R}{D}G(\boldsymbol{x}^a|\boldsymbol{x}^s) \tag{S2}$$

where $G(\boldsymbol{x}^a|\boldsymbol{x}^s)$ is the Green's function of the Helmholtz operator $\nabla^2 + k^2$ with $k = \mathrm{i}/\sqrt{D\tau}$. Explicitly, the solution reads, for any number of dimensions $n$,

$$c(\boldsymbol{x}^a|\boldsymbol{x}^s) = \frac{R}{D}\frac{1}{(2\pi)^{n/2}}\left(\frac{1}{\lambda d}\right)^{n/2-1} K_{n/2-1}(d/\lambda) \tag{S3}$$

where $d = \|\boldsymbol{x}^s - \boldsymbol{x}^a\|_2$, where $\lambda = \sqrt{D\tau}$ is a characteristic lengthscale for dispersion, and where $K_\nu$ is the modified Bessel function of the second kind of order $\nu$.

In particular

$$n = 1: \qquad c(\boldsymbol{x}^a|\boldsymbol{x}^s) = \frac{R}{D}\frac{\lambda}{2}\exp(-d/\lambda), \tag{S4a}$$

$$n = 2: \qquad c(\boldsymbol{x}^a|\boldsymbol{x}^s) = \frac{R}{D}\frac{1}{2\pi}K_0(d/\lambda), \tag{S4b}$$

$$n = 3: \qquad c(\boldsymbol{x}^a|\boldsymbol{x}^s) = \frac{R}{D}\frac{1}{4\pi d}\exp(-d/\lambda). \tag{S4c}$$

## 1.2 Model of detection

We now derive the mean number of odor particles detected by the agent using a simple model of chemoreception in the neighborhood of the agent (far from the source) based on the assumption that the agent acts as a perfect sink for those particles.

Consider an agent modeled as an $n$-ball (ball of dimension $n$) with radius $a$ in a medium with diffusion lengthscale $\lambda \gg a$. Suppose that the agent surface is fully covered in receptors, and that every particle that reaches the surface is absorbed, such that the concentration on the ball surface is zero. Far from the agent, the concentration field is $c_\infty$. In a frame of reference center on the agent, and introducing $\rho$ as the distance to the origin, the stationary concentration $c$ in the near-field satisfies

$$\nabla^2 c = 0 \qquad \text{with } \nabla^2 = \partial_\rho^2 + \frac{n-1}{\rho}\partial_\rho \tag{S5}$$

with boundary conditions

$$c(\rho = a) = 0, \qquad c(\rho \to \lambda) \to c_\infty. \tag{S6}$$

Note that the introduction of the cut-off lengthcale $\lambda$ in the second boundary condition is required to regularize the solution in 1D and 2D, which otherwise diverges.

The solution is

$$n = 1: \qquad c(\rho) = \frac{c_\infty}{\lambda - a}(\rho - a), \tag{S7a}$$

$$n = 2: \qquad c(\rho) = \frac{c_\infty}{\ln(\lambda/a)}\ln(\rho/a), \tag{S7b}$$

$$n = 3: \qquad c(\rho) = c_\infty\left[1 - \left(\frac{a}{\rho}\right)\right], \tag{S7c}$$

$$n \geqslant 3: \qquad c(\rho) = c_\infty\left[1 - \left(\frac{a}{\rho}\right)^{n-2}\right]. \tag{S7d}$$

The total flux toward the agent corresponds to the average number of particles which, due to their random motion, collide with its surface and are absorbed per unit time. It reads

$$J = D \left. \frac{\mathrm{d}c}{\mathrm{d}\rho} \right|_{\rho=a} S_n \tag{S8}$$

where $S_n$ is the surface area of the $n$-ball

$$S_n = \frac{2\pi^{n/2} a^{n-1}}{\Gamma(n/2)} \tag{S9}$$

with $\Gamma$ the gamma function. Explicitly this reads

$$n = 1: \qquad J = 2D \frac{c_\infty}{\lambda - a}, \tag{S10a}$$

$$n = 2: \qquad J = 2\pi D \frac{c_\infty}{\ln(\lambda/a)}, \tag{S10b}$$

$$n = 3: \qquad J = 4\pi a D c_\infty, \tag{S10c}$$

$$n \geqslant 3: \qquad J = \frac{2\pi^{n/2}(n-2)a^{n-2}}{\Gamma(n/2)} D c_\infty. \tag{S10d}$$

## 1.3 Mean number of hits

The expressions for the flux and for the mean field concentration can be matched by requiring that $c_\infty = c(\boldsymbol{x}^a|\boldsymbol{x}^s)$. The mean number of particles detected during a time $\Delta t$ is $\mu = J\Delta t$, which yields the expressions given in the main document and repeated hereafter:

$$n = 1: \qquad \mu(d) = R\Delta t \frac{\lambda}{\lambda - a} \exp(-d/\lambda), \tag{S11a}$$

$$n = 2: \qquad \mu(d) = R\Delta t \frac{1}{\ln(\lambda/a)} K_0(d/\lambda), \tag{S11b}$$

$$n = 3: \qquad \mu(d) = R\Delta t \frac{a}{d} \exp(-d/\lambda), \tag{S11c}$$

$$n = 4: \qquad \mu(d) = R\Delta t \left(\frac{a}{\lambda}\right)^2 \frac{\lambda}{d} K_1(d/\lambda), \tag{S11d}$$

$$n \geqslant 3: \qquad \mu(d) = R\Delta t \left(\frac{a}{\lambda}\right)^{n-2} \left(\frac{\lambda}{d}\right)^{n/2-1} \frac{(n-2)}{\Gamma(n/2)} \frac{K_{n/2-1}(d/\lambda)}{2^{n/2-1}}. \tag{S11e}$$

Examples of hit distributions and their mean as a function of the distance to the source are shown in Fig. S1.

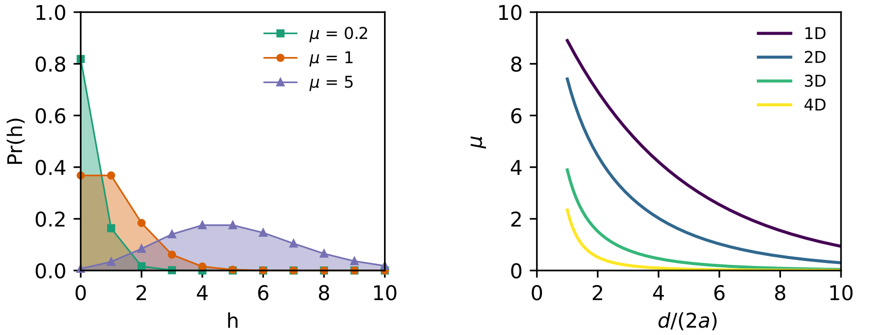


**Figure S1** Illustration of the detection model: hits $h$ are distributed according to a Poisson's law parameterized by its mean $\mu$, which is a decreasing function of the Euclidean distance $d$ to the source, and which functional form depends on the problem dimensionality (here $\lambda/a = 8$ and $R\Delta t = 10$).

# 2 Additional information on our methodology

## 2.1 Numerical parameters summary

The values of the numerical parameters used in our study are summarized in Table S1.

| dimension | $\varepsilon_{\text{out}}$ | $\varepsilon_{\text{stop}}$ | $\varepsilon_{\text{acc}}$ | $N_{\text{stuck}}$ | number of episodes |
|---|---|---|---|---|---|
| 1D | $10^{-3}$ | $10^{-6}$ | $10^{-10}$ | 8 | $\geqslant 16000$ |
| 2D | $10^{-3}$ | $10^{-6}$ | $10^{-10}$ | 8 | $\geqslant 6400$ |
| 3D | $10^{-3}$ | $10^{-6}$ | $10^{-10}$ | 8 | $\geqslant 25600$ |
| 4D | $10^{-3}$ | $10^{-6}$ | $10^{-10}$ | 8 | [1024,4096] |

**Table S1** Summary of numerical parameters used to compute statistics: $\varepsilon_{\text{out}}$ determines the size of the numerical domain, $\varepsilon_{\text{stop}}$ defines the stopping criteria in the hybrid Bayesian/Monte-Carlo approach, $\varepsilon_{\text{acc}}$ is the numerical accuracy used to determine whether two actions are equivalent, and $N_{\text{stuck}}$ provides a criteria to declare that the agent is stuck in an infinite loop. The number of episodes is chosen such that the mean of the distribution is well-converged, with a 95% confidence interval less than ±2% in 1D to 3D (accuracy is lower in 4D due to the high cost of the simulations).

## 2.2 Initialization protocol

The procedure we use to determine a "large enough" domain size is explained in the main document (appendix). It essentially yields $N \propto \mathcal{L}$ with a proportionality constant that depends on $\varepsilon_{\text{out}}$ (and weakly on $\mathcal{I}$), as shown in Fig. S2.

We used $\varepsilon_{\text{out}} = 10^{-3}$ for all the simulations presented in the main document. This particular value of $\varepsilon_{\text{out}}$ was determined from preliminary tests showing that the mean time to find the source with the infotaxis policy has converged to a constant independent of $\varepsilon_{\text{out}}$ for $n > 1$ (in 1D and in the absence of hits, infotactic agents tend to go to one end of the domain before turning back, therefore the mean time to find the source does not converge with the domain size).

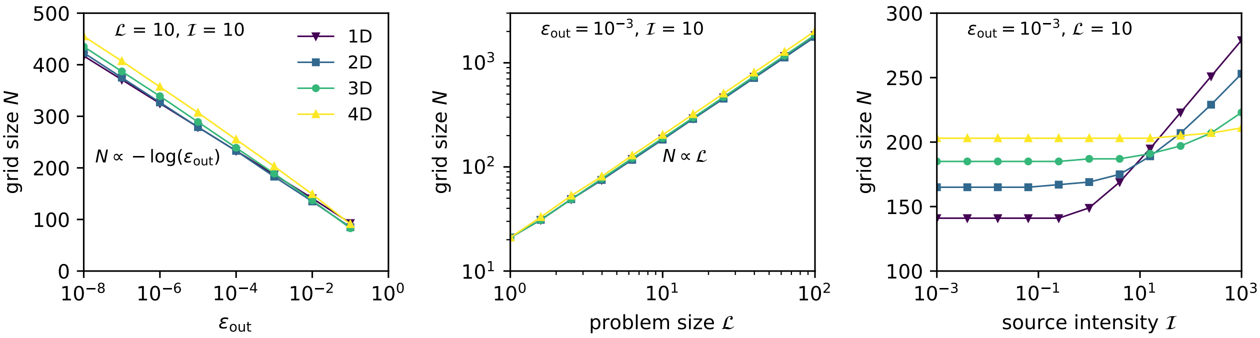


**Figure S2** Initialization procedure: grid size as a function of $\varepsilon_{\text{out}}$, $\mathcal{L}$ and $\mathcal{I}$ when following our methodology.

## 2.3 Policy evaluation

Policy evaluation is performed by generating a large number of episodes and computing the resulting distribution of arrival times $T$, denoted here $f(T)$, and defined such that its norm is the probability of (ever) finding the source (which may not be equal to one), that is,

$$\Pr(\text{failure}) = 1 - \sum_T f(T). \tag{S12}$$

Other moments of the distribution are computed after renormalization as usual:

$$\text{Mean}(T) = \sum_T T\tilde{f}(T), \qquad \text{Std}(T) = \sqrt{\sum_T T^2\tilde{f}(T) - \text{Mean}(T)^2} \qquad \text{with } \tilde{f}(T) = \frac{f(T)}{\sum_T f(T)}. \tag{S13}$$

We compute $f(T)$ using our hybrid Bayesian/Monte-Carlo framework, which allows us to sample the tail of the distribution more efficiently than with standard Monte-Carlo simulations. In this framework, episodes are independent of the true source location: the search continues until the probability of having found the source is equal to one (within numerical accuracy $\varepsilon_{\text{stop}}$) or until the agent is stuck in an infinite loop, and the hits are drawn at each step according to

$$\Pr(h|\boldsymbol{x}^a) = \sum_{\boldsymbol{x}} \Pr(h|\boldsymbol{x}^a, \boldsymbol{x}) p(\boldsymbol{x}). \tag{S14}$$

The pseudo-code for computing the distribution of arrival times $f(T)$ using the hybrid Bayesian/Monte-Carlo method is given in Fig. S3. The numerical proof of its correctness and efficiency, compared to full Monte-Carlo, is given in Fig. S4: both methods ultimately yield the same distributions (top row), but the hybrid method converges faster and is well-suited for probing rare events, such as the probability of never finding the source (bottom row).

We use $\varepsilon_{\text{stop}} = 10^{-6}$ (unless mentioned otherwise): this means that the search continues until the probability that the source has not been found is less than $10^{-6}$. We found that this value was sufficiently low to obtain very clean statistics of the arrival times (in particular of the tail of their distribution) while keeping the computational cost acceptable.

```
pdf[i] ← 0 for all i                          // probability density function f(T) to be filled
Nepisodes ← 0
converged_stats ← False
while not converged_stats do
    Nepisodes ← Nepisodes + 1
    agent ← init_agent()                                // agent position x^a
    p_source ← init_p_source()                // source probability distribution p(x)
    t ← 0
    agent_stuck ← False
    p_not_found_yet ← 1.0            // probability that the source has not been found yet
    episodic_pdf[i] ← 0 for all i              // pdf of arrival times for this episode
    while p_not_found_yet > ε_stop and not agent_stuck do
        t ← t + 1
        action ← policy(agent, p_source)
        agent ← move(agent, action)
        p_end ← p_source[agent]        // probability that the source is in the agent's cell
        episodic_pdf[t] ← p_not_found_yet * p_end
        p_not_found_yet ← p_not_found_yet * (1.0 − p_end)
        p_source ← Bayes_update_after_source_not_found(agent, p_source)
        hit ← draw_random_hit(agent, p_source)              // according to Eq.  (S14)
        p_source ← Bayes_update_after_hit_received(agent, p_source, hit)
        agent_stuck ← is_agent_stuck()
    end while
    pdf[i] ← pdf[i] + episodic_pdf[i] for all i
    converged_stats ← are_stats_converged()
end while
pdf[i] ← pdf[i]/Nepisodes for all i             // compute f(T) by averaging over episodic pdfs
return pdf
```

**Figure S3** Pseudo-code for efficient computation of probability density function $f(T)$ with our hybrid Bayesian/Monte-Carlo method. The norm of $f(T)$ is the probability of (ever) finding the source.

## 2.4 Other implementation details

Parts of the computations involve a summation over all possible hit values (more generally, over all possible successor belief states). A natural way to compute this summation would consist in keeping adding terms associated to increasing hit values until the desired accuracy is reached. However, for computational efficiency, we found desirable to set this cut-off value to a constant. In particular, Eq. (S14) can be viewed as a tensor dot product, and can be computed efficiently by storing $\Pr(h|\boldsymbol{x}^a, \boldsymbol{x})$ for all possible values of $h$ beforehand. We remind the reader that $h$ is a random variable following a Poisson distribution with mean (and variance) $\mu(d)$ where $\mu$ is a decreasing function of the distance $d$ between the agent and the source. The cut-off value was therefore set to $\text{Mean}(h) + \text{Std}(h)$ at a distance $\Delta x$ from the source, that is $h_{\max} = \mu(\Delta x) + \sqrt{\mu(\Delta x)}$. Note that

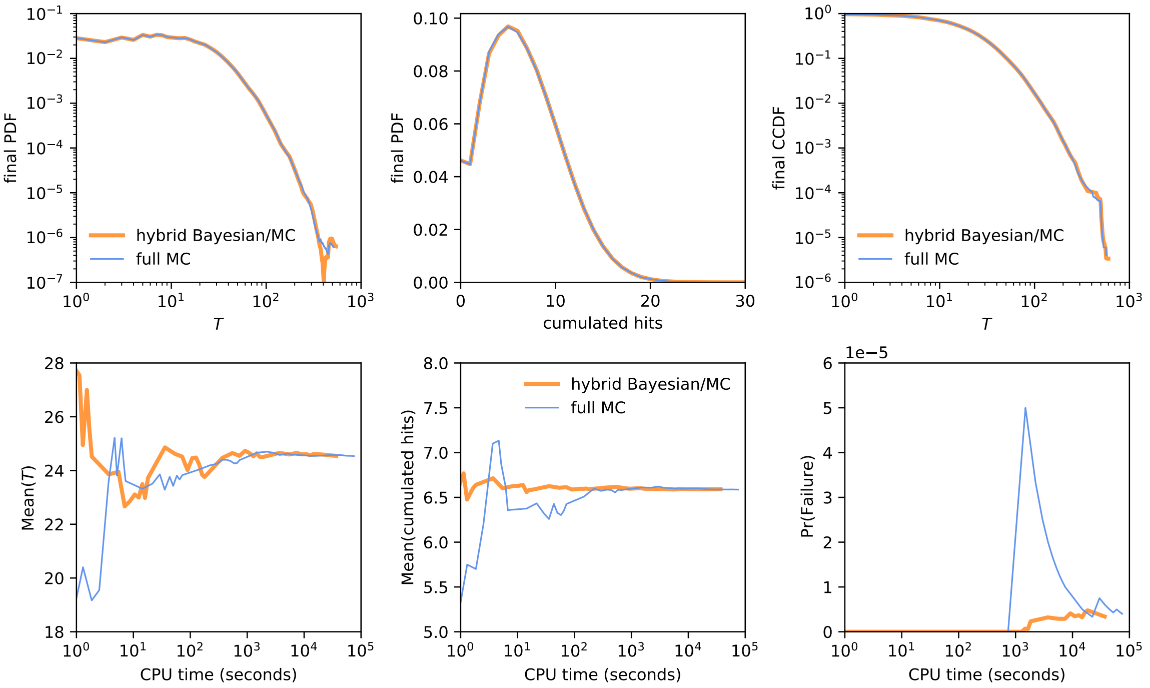


**Figure S4** Comparison of full Monte-Carlo and hybrid Bayesian/Monte-Carlo methods (here with $\varepsilon_{\text{stop}} = 10^{-10}$) for computing the statistics of a policy. PDF stands for probability density function (which shows the probability of finding the source in $T$ steps), and CCDF stands for complementary cumulative distribution function (which shows the probability of the source not being found after $T$ steps). The number of cumulated hits does not include the initial hit used to define the start of the search. A total of $10^6$ and $2 \times 10^5$ episodes were used for the full Monte-Carlo and the hybrid Bayesian/Monte-Carlo methods, respectively. These simulations used the infotaxis policy in 2D with $\mathcal{L} = 2$ and $\mathcal{I} = 2$.

$d = \Delta x$ is the minimal distance between the agent and the source ($\mu$ is not defined for $d = 0$ since this would mean that the source is found). We ensured that this cut-off value was large enough not to affect our results.

Even with deterministic policies, the choice of action is not unique in case of ties. Consider for example the choice of the first action: all actions are equivalent due to the symmetries of the problem. However, due to finite numerical accuracy, these symmetries may be broken artificially. On the other hand, numerical accuracy can generate artificial ties later in the search. Consider for example the infotaxis policy which consists in choosing the action that minimizes the expected entropy of the next belief state. Close to the end of the search, the entropy may be very low, and numerically indistinguishable from zero, leading to “wrong” choices. To ensure reproducibility of our results, we control the numerical accuracy by introducing a small parameter $\varepsilon_{\text{acc}}$. We assume that two actions are equivalent if the criteria used by the policy to evaluate them (for example the expected entropy for infotaxis or the expected optimal value for the optimal policy) are equal within $\varepsilon_{\text{acc}} = 10^{-10}$.

Common practice consists in breaking ties randomly. Here we chose instead to break ties in a deterministic manner: when ’east’ and ’west’ are equivalent, the chosen action will always be ’east’. This allows us to easily identify situations where the agent is lost (in the sense that the policy can no longer discriminate between actions, for example because the agent ventured too far from the source): with our setup, a lost agent will be trapped in an infinite loop which is trivial to detect and allows us to stop the simulation. In contrast, with random tie-breaking, a lost agent would perform a random walk, which is of no interest for the problem we consider and would waste huge computational resources (think how long it takes to explore a 4D space with a random walk).

Rigorously speaking, infinite loops in the agent displacements may not be truly infinite, since they may be broken by a lucky hit if one waits long enough. These finite loops essentially amount to waiting for such a lucky hit to happen, and their presence always degrade performance, therefore we declare the agent as stuck and stop the search when a “long enough” loop is encountered. More precisely, the agent is stuck if $\boldsymbol{x}^a_t = \boldsymbol{x}^a_{t-2}$ more than $N_{\text{stuck}}$ times in a row. We used $N_{\text{stuck}} = 8$ in our simulations. The particular choice of $N_{\text{stuck}}$ has no effect on the performance we report for good policies such as infotaxis and its derivatives, since they are not prone to such loops. It may however affect our measure of performance for policies which systematically generates loops (such as those presented in Section 3). It is unimportant though, since such policies are always poor.

# 3 Naive policies

In this section we report on the performance of "naive" policies on the source-tracking problem. We remind the reader that a policy is a mapping from belief state $s$ to action $a$, where the belief state is $s = [\boldsymbol{x}^a, p(\boldsymbol{x})]$ with $\boldsymbol{x}^a$ the agent's position and $p(\boldsymbol{x})$ the probability distribution of source locations. For each possible action corresponds a new deterministic position which we denote $\boldsymbol{x}^a(a)$.

We first consider the usual "greedy" policy, defined as the short-sighted exploitative policy that minimizes the penalty at the next step. In the source tracking problem, the greedy policy consists in choosing the action that maximizes the probability of finding the source in the next cell:

$$\pi^{\text{greedy}}(s) = \underset{a}{\arg\max}\, p(\boldsymbol{x}^a(a)). \tag{S15}$$

The probability of failure with the greedy policy is plotted in Fig. S5(a) for 2D searches. In the absence of cues ($\mathcal{I} \to 0$), the greedy policy performs well because it behaves as an exhaustive search, spiraling outward from the center of the domain. However in the presence of cues the greedy agent is often lost, with Pr(failure) greater than 1 % or even 10 %. This is due to the locality of the greedy policy (the greedy agent chooses its action based only on $p(\boldsymbol{x})$ around itself) which tends to trap the agent in a neighborhood of vanishing $p(\boldsymbol{x})$. Unable to choose a meaningful action, the greedy agent then heads to the domain boundaries, as illustrated in accompanying videos (cf. Section 9).

We then consider three policies that would be optimal in the absence of uncertainty, since they would all direct the agent to the (known) source location.

The first one is the "most likely state (mls)" policy [1] which finds the most likely source location, and executes the action that would be optimal for that location. In other words, the agent executing this policy moves in the direction of the most likely source location. This reads

$$\pi^{\text{mls}}(s) = \underset{a}{\arg\min} \|\boldsymbol{x}^{\text{mls}} - \boldsymbol{x}^a(a)\|_1 \tag{S16}$$

where $\boldsymbol{x}^{\text{mls}}$ is the most likely source location

$$\boldsymbol{x}^{\text{mls}} = \underset{\boldsymbol{x}}{\arg\max}\, p(\boldsymbol{x}). \tag{S17}$$

Another possibility is the "voting" policy [1] which chooses the action that is the most likely to be optimal. For that, it determines the optimal action for each possible source location, weights each action by the corresponding probability of that location being the true source location, and picks the action with the highest probability. The probability that action $a$ is optimal is

$$w(a) = \sum_{\boldsymbol{x}} \Pr(\boldsymbol{x}) \phi(a^*(\boldsymbol{x}) = a) \tag{S18}$$

where $\phi$ has value 1 if the argument is true and 0 otherwise, and where $a^*(\boldsymbol{x})$ denote the optimal action for a source located in $\boldsymbol{x}$, which is given by

$$a^*(\boldsymbol{x}) = \underset{a}{\arg\min} \|\boldsymbol{x} - \boldsymbol{x}^a(a)\|_1. \tag{S19}$$

The voting policy then reads

$$\pi^{\text{voting}}(s) = \underset{a}{\arg\max}\, w(a). \tag{S20}$$

We finally consider a policy based on the intuitive idea that the agent should get, on average, closer to the source. For a belief state $s = [\boldsymbol{x}^a, p(\boldsymbol{x})]$, the mean distance to the source is denoted $D$ and defined by

$$D(s) = \sum_{\boldsymbol{x}} p(\boldsymbol{x}) \|\boldsymbol{x} - \boldsymbol{x}^a\|_1. \tag{S21}$$

where we used the Manhattan norm (other norms would yield similar results). The expected value of this mean distance upon executing action $a$ in belief state $s$ is given by

$$D(s|a) = \sum_{s'} \Pr(s'|s, a) D(s') \tag{S22}$$

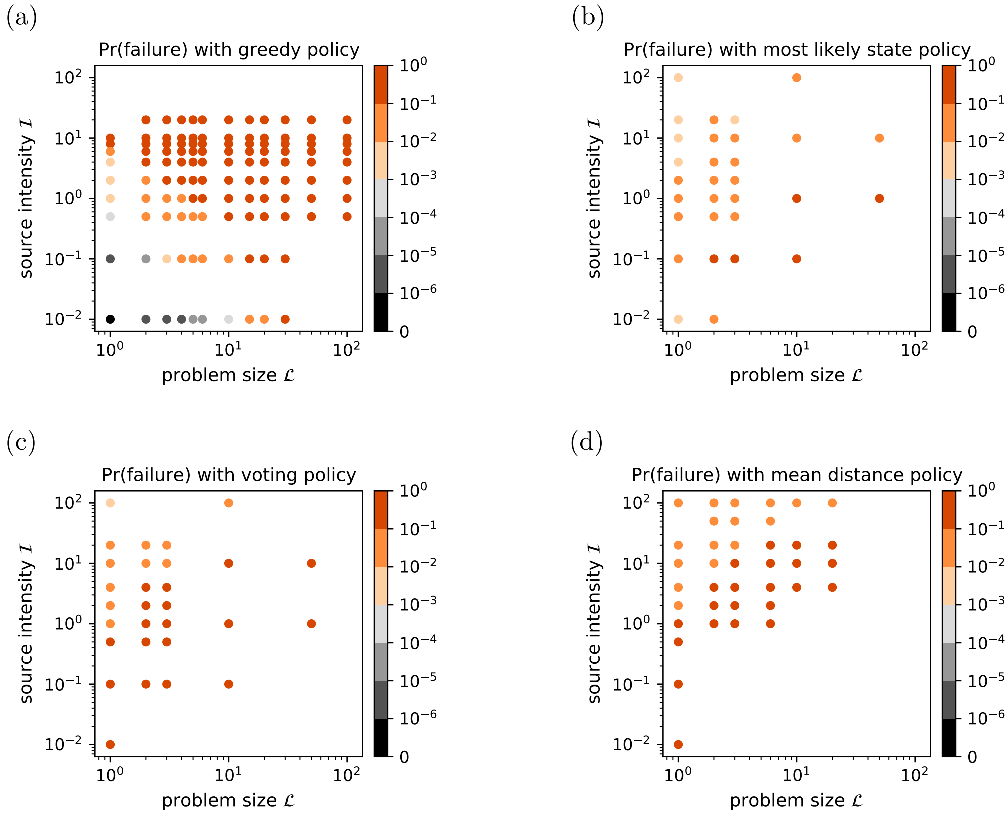


**Figure S5** Probability of never finding the source in 2D for (a) the greedy policy, (b) the most likely state policy, (c) the voting policy and (d) the mean distance policy, as a function of the problem size $\mathcal{L}$ and source intensity $\mathcal{I}$.

where the sum is taken over all successor belief states $s'$. The "mean distance" policy is then defined by

$$\pi^{\text{mean distance}}(s) = \arg\min_a D(s|a) \tag{S23}$$

and consists in choosing the action that minimizes the expected distance to the source at the next step. Besides, for any belief state, the mean Manhattan distance is a lower bound for the optimal value $v^*(s)$ ($D(s) \leqslant v^*(s)$). The mean distance policy therefore minimizes the expected lower bound of the optimal value function.

The probabilities of failing to find the source in 2D with the most-likely-state, voting and mean-distance policies are shown in Fig. S5(b,c,d). Reliability is very poor for the entire range of parameters, with Pr(failure) always greater than 0.1 %, and often larger than 1 % or even 10 %. This is because an agent following any of those policies gets systematically trapped in loops early on during the search. The emergence of these loops is due to high degree of symmetry in $p(\boldsymbol{x})$ (itself due to the lack of directionality in the information provided by hits), as illustrated in accompanying videos (cf. Section 9).

# 4 Explicit calculation of the expected entropy

Infotaxis (and space-aware infotaxis) requires the computation of the entropy upon taking action $a$ in belief state $s$, denoted $H(s|a)$ in the main document. Here we consider an explicit example to show how $H(s|a)$ is calculated.

Suppose that the agent is currently in belief state $s_t = [\boldsymbol{x}_t^a, p_t(\boldsymbol{x})]$, and consider an action $a_t$ that would move the agent to a new position $\boldsymbol{x}_{t+1}^a$. Possible outcomes are

- with probability $p_t(\boldsymbol{x}_{t+1}^a)$, the agent will find the source and the new belief state will be $s^\Omega$ with $H(s^\Omega) = 0$,
- with probability $1 - p_t(\boldsymbol{x}_{t+1}^a)$, the agent will not find the source, and $p_t(\boldsymbol{x})$ will be updated to $\tilde{p}_t(\boldsymbol{x}) = \text{Bayes}(p_t(\boldsymbol{x}), \boldsymbol{x}_{t+1}^a, \bar{F})$ (a simple renormalization to account for the absence of the source). We denote this intermediate belief state $\tilde{s}_t = [\boldsymbol{x}_{t+1}^a, \tilde{p}_t(\boldsymbol{x})]$. Then the agent will receive a hit $h_t$. Possible outcomes are:
  - the agent will receive 0 hit with probability $\Pr(h_t = 0|\boldsymbol{x}_{t+1}^a)$, update the posterior to $p_{t+1}^0(\boldsymbol{x}) = \text{Bayes}(\tilde{p}_t(\boldsymbol{x}), \boldsymbol{x}_{t+1}^a, 0)$ and the new belief state will be $s_{t+1}^0 = [\boldsymbol{x}_t^a, p_{t+1}^0(\boldsymbol{x})]$ with entropy $H(s_{t+1}^0)$,
  - the agent will receive 1 hit with probability $\Pr(h_t = 1|\boldsymbol{x}_{t+1}^a)$, and similarly the new belief state will be $s_{t+1}^1 = [\boldsymbol{x}_t^a, p_{t+1}^1(\boldsymbol{x})]$ with entropy $H(s_{t+1}^1)$,
  - etc.

as illustrated in Fig. S6. The probability of each hit value is given by

$$\Pr(h_t|\boldsymbol{x}_{t+1}^a) = \sum_{\boldsymbol{x}'} \Pr(h_t|\boldsymbol{x}_{t+1}^a, \boldsymbol{x}')\tilde{p}_t(\boldsymbol{x}'). \tag{S24}$$

The expected entropy upon taking action $a_t$ in belief state $s_t$ is therefore

$$H(s_t|a_t) = p_t(\boldsymbol{x}_{t+1}^a) \cdot 0 + \left[1 - p_t(\boldsymbol{x}_{t+1}^a)\right] \left[\sum_{h_t} \Pr(h_t|\boldsymbol{x}_{t+1}^a) H(s_{t+1}^{h_t})\right]. \tag{S25}$$

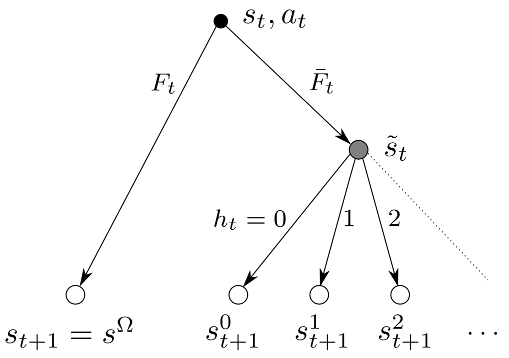


**Figure S6** Tree of possible successor belief states $s_{t+1}$ starting from a belief state $s_t$ and executing action $a_t$. Transitions from $s_t$ to $s_{t+1}$ are determined by the observations: either finding the source ($F_t$) or not finding the source ($\bar{F}_t$) and receiving $h_t$ hits.

# 5 Additional results on infotaxis

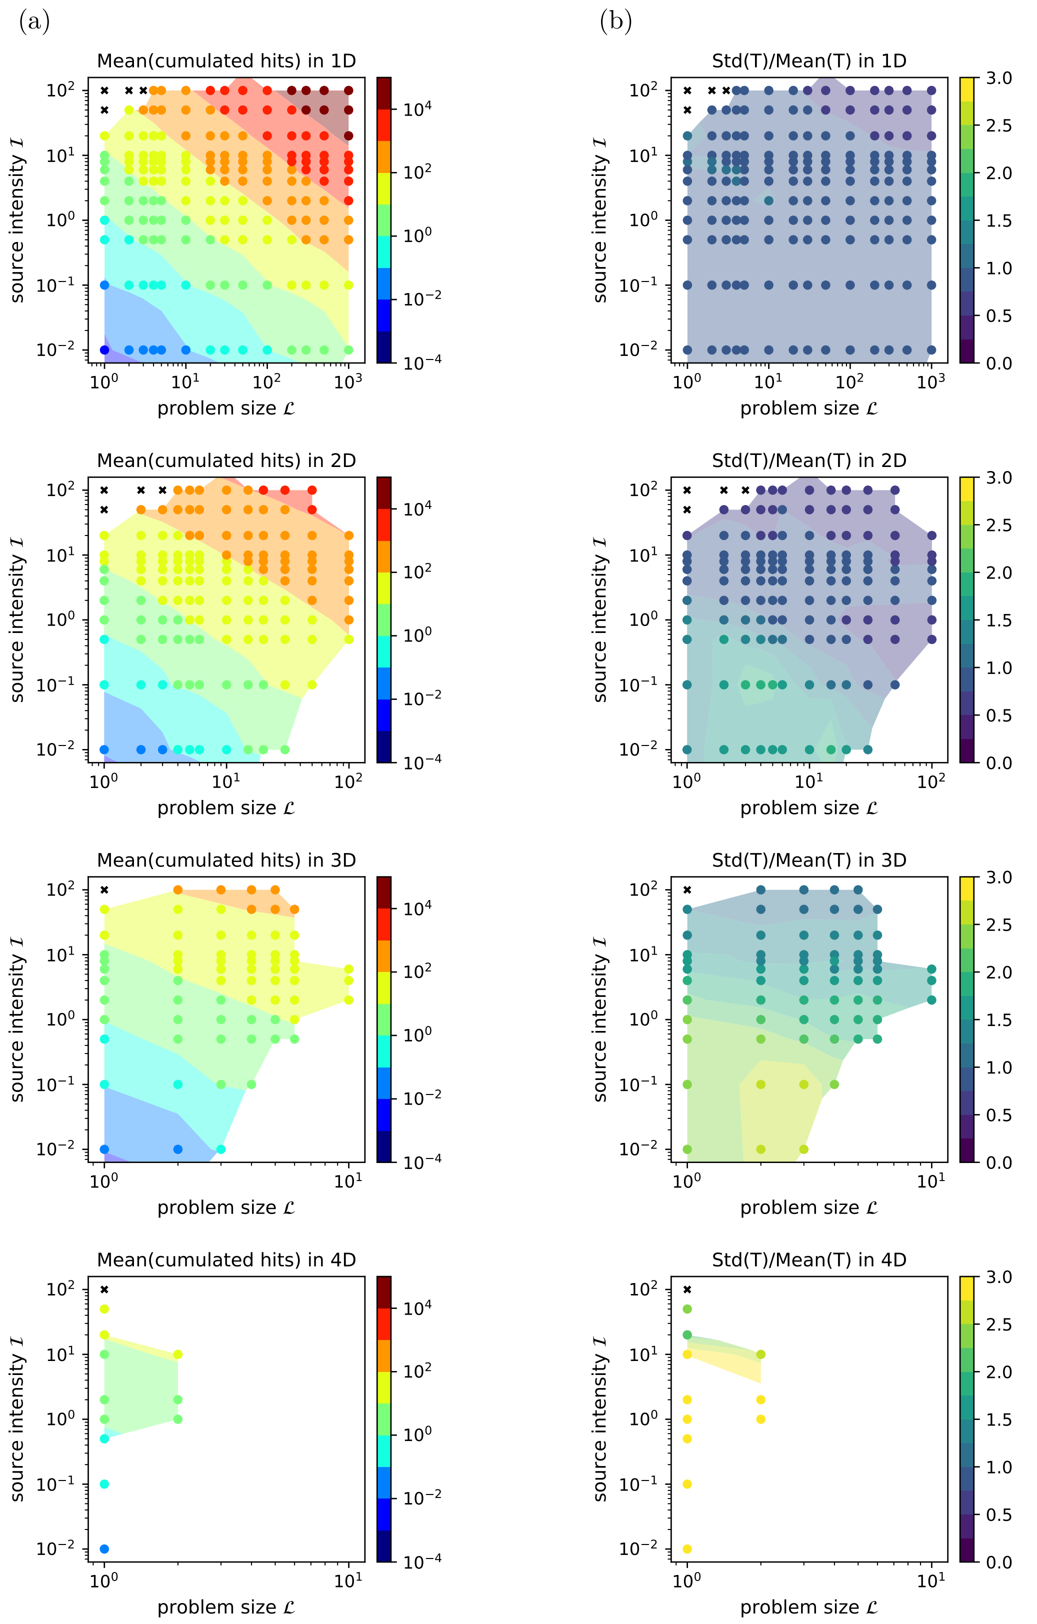


**Figure S7** Additional statistics of infotactic searches for source tracking in 1D, 2D, 3D and 4D (rows), for a wide range of physical parameters $\mathcal{L}$ and $\mathcal{I}$: (a) mean number of cumulated hits to find the source (excluding the initial one) and (b) standard deviation of arrival times distribution normalized by its mean. The crosses depict cases where $\Pr(\text{failure}) > 10^{-3}$.

# 6 N-step infotaxis algorithm

In this section we give the algorithm for N-step infotaxis. Let us first consider 2-step infotaxis, which consists in choosing the action that maximizes the expected gain of information after executing two actions. Formally, this reads

$$\pi^{\text{2-step infotaxis}}(s) = \underset{a}{\arg\max} \left\{ G(s,a) + \gamma \sum_{s'} \Pr(s'|s,a) \max_{a'} G(s',a') \right\} \tag{S26}$$

where $\gamma$ is a discount factor which we will discuss later on, and which controls the weight given to the gain expected from the second action compared to that from the first action.

The expression given by Eq. (S26) is better understood from Fig. S8, which illustrates how it is calculated. First, we expand the tree from belief state $s$ (top node) and calculate all possible belief states $s''$ (bottom nodes) that can be reached after executing any combination of two actions $a$ and $a'$. Each of these belief states has an associated entropy $H(s'')$. Then, we transfer this information back to the top node through successive reduction operations as follows (this procedure is sometimes called "backup" in tree-search planning and reinforcement learning) :

1. for each node $s''$ we calculate its entropy $H(s'')$;
2. for each node $a'$ we can calculate the expected gain $G(s',a') = H(s') - H(s'|a)$ where $H(s'|a') = \sum_{s''} \Pr(s''|s',a')H(s'')$;
3. for each node $s'$ we choose the infotactic action that maximizes $G(s'|a')$, that is, we associate each node $s'$ to $\max_{a'} G(s'|a')$;
4. for each node $a$ we can calculate the gain $G(s,a)$ expected from action $a$, as well as the maximum gain expected from action $a'$ which reads $\sum_{s'} [\Pr(s'|s,a) \max_{a'} G(s'|a')]$, and we then associate each node $a$ to the expected discounted cumulated gain $G(s,a) + \gamma \sum_{s'} [\Pr(s'|s,a) \max_{a'} G(s'|a')]$;
5. minimizing this last expression over actions $a$ takes us back to the starting node $s$ and yields Eq. (S26).

The generalization to $N_{\text{steps}}$ steps is straightforward from Fig. S8.

We now come back to the introduction of a discount factor, with $0 \leqslant \gamma \leqslant 1$. Discounting with factor $\gamma$ means that an information gain received at the i-th step is worth only $\gamma^{i-1}$ times what it would be worth at the first step, and translates the idea that gaining an amount now is better than gaining the same amount later. If $\gamma = 0$, all later gains are entirely discounted and one recovers (1-step) infotaxis. If $\gamma = 1$, all later gains have the same weight as the first one. This is not desirable, because this means, for example, that in a situation where the source can be surely found in either 1 or 3 steps, 3-step infotaxis would consider both options equal. In our numerical experiments we used $\gamma = 0.999$, which alleviates the above-mentioned issue without discarding information from the deepest layers of the tree. Note that without discount ($\gamma = 1$), the algorithm simplifies and is given in [2].

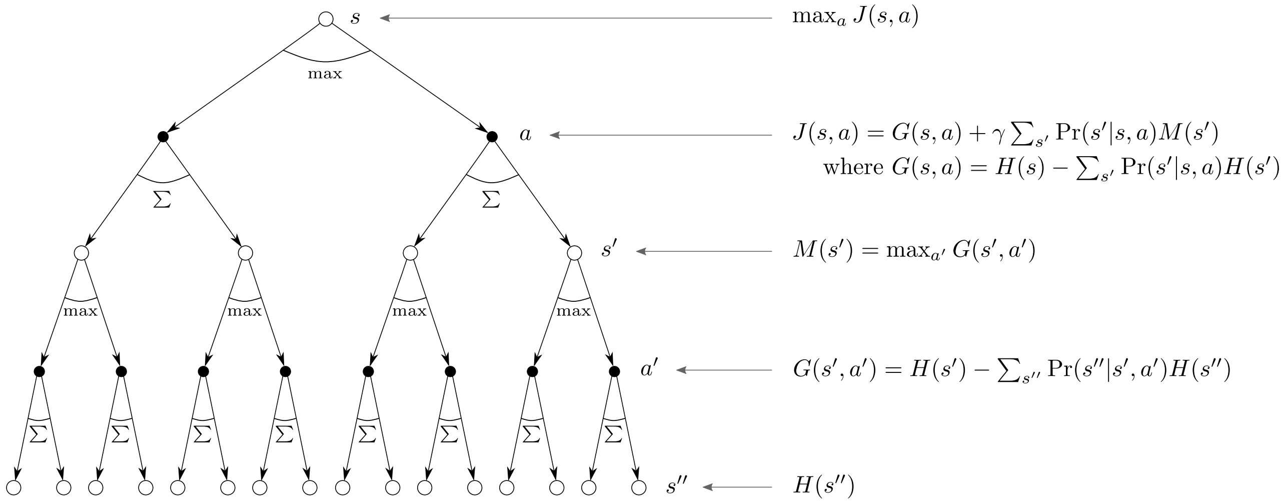


**Figure S8** Backup diagram for 2-step infotaxis.

# 7 Additional results on space-aware infotaxis

With space-aware infotaxis (SAI), the agent chooses the action that minimizes the expectation of

$$J(s) = \log_2\left(D(s) + 2^{H(s)-1} - \frac{1}{2}\right) \tag{S27}$$

at the next step, where $H(s)$ is the entropy of belief state $s$ and $D(s)$ is the mean Manhattan distance between the agent and the source. The distribution of arrival times with SAI is shown in Fig. S9. The standardized distributions of arrival times exhibit the same features as those obtained with infotaxis (cf. main document). The only significant differences are the oscillations in the distribution of the 1D arrival times, particulary visible for small domains: they are the signature of the back-and-forth trajectories of SAI in 1D.

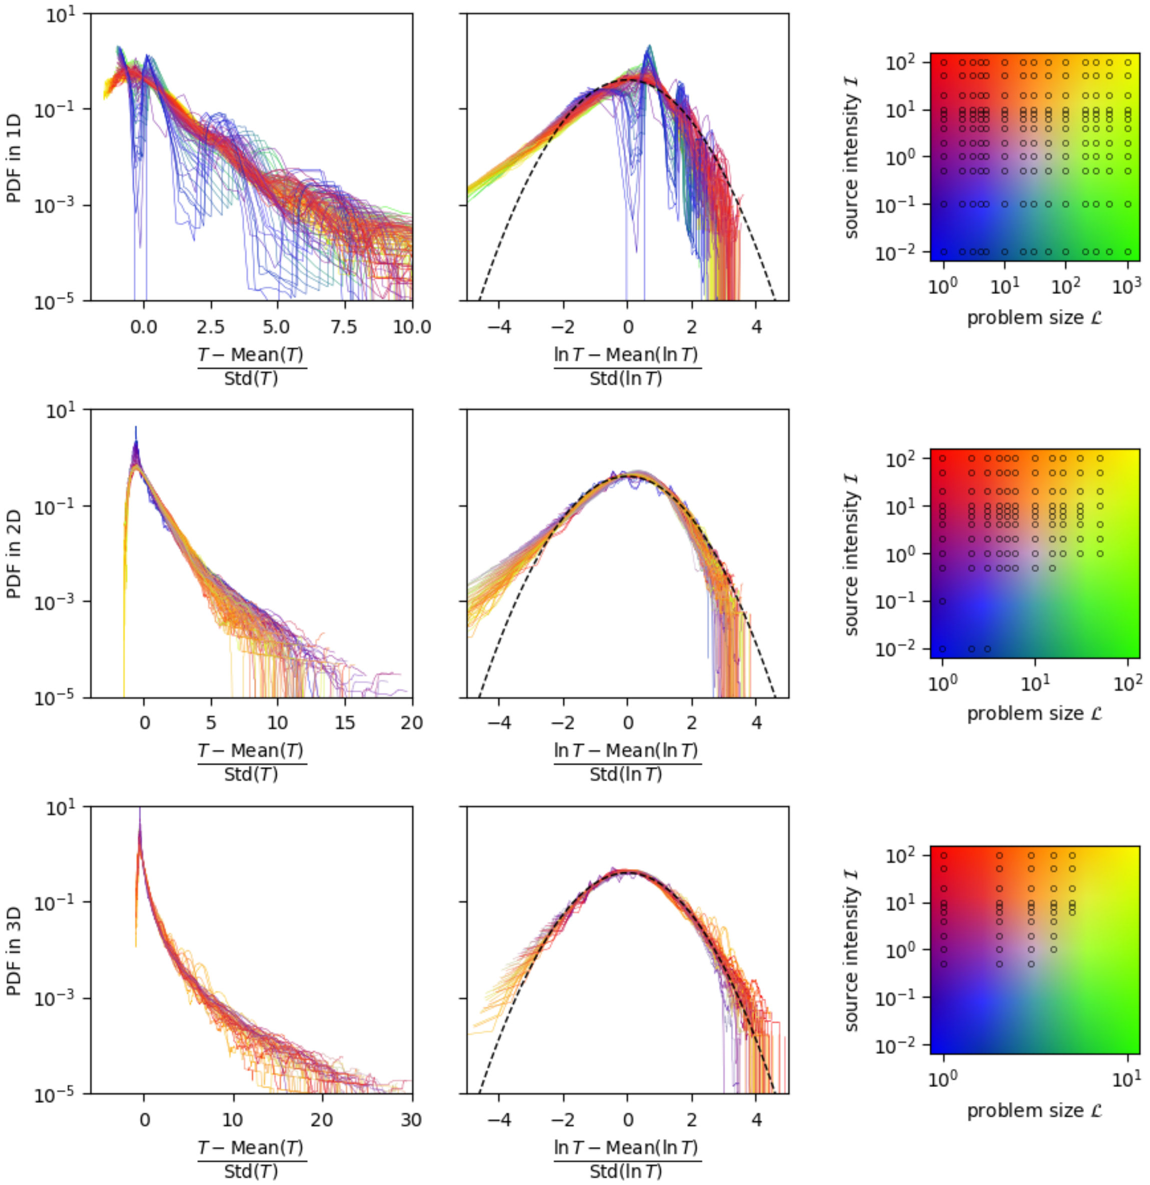


**Figure S9** Distributions of arrival times with space-aware infotaxis (SAI) for source tracking in 1D, 2D and 3D (rows) for a wide range of problem sizes $\mathcal{L}$ and source intensities $\mathcal{I}$ (color-coded according to the map on the right). The same data is plotted in both columns using different scales to evidence the distribution features. The dashed line (right column) shows a standardized log-normal distribution.

While the choice of the Manhattan norm in the definition of $D$ is the most intuitive, the Euclidean norm is also a natural candidate since it determines the occurrence of hits. In more than 1D, this choice may matter. Therefore we evaluated the performance of an alternative version, SAI-2, that uses the mean Euclidean distance between the agent and the source as the definition for $D$:

$$D(s) = \sum_{\boldsymbol{x}} p(\boldsymbol{x}) \|\boldsymbol{x} - \boldsymbol{x}^a\|_2 \tag{S28}$$

where $p(\boldsymbol{x})$ is the probability of the source being in $\boldsymbol{x}$ and $\boldsymbol{x}^a$ is the agent location. The results, presented in Fig. S10, show that SAI-2 performs well, although marginally worse than SAI (the version based on the Manhattan norm, cf. main document).

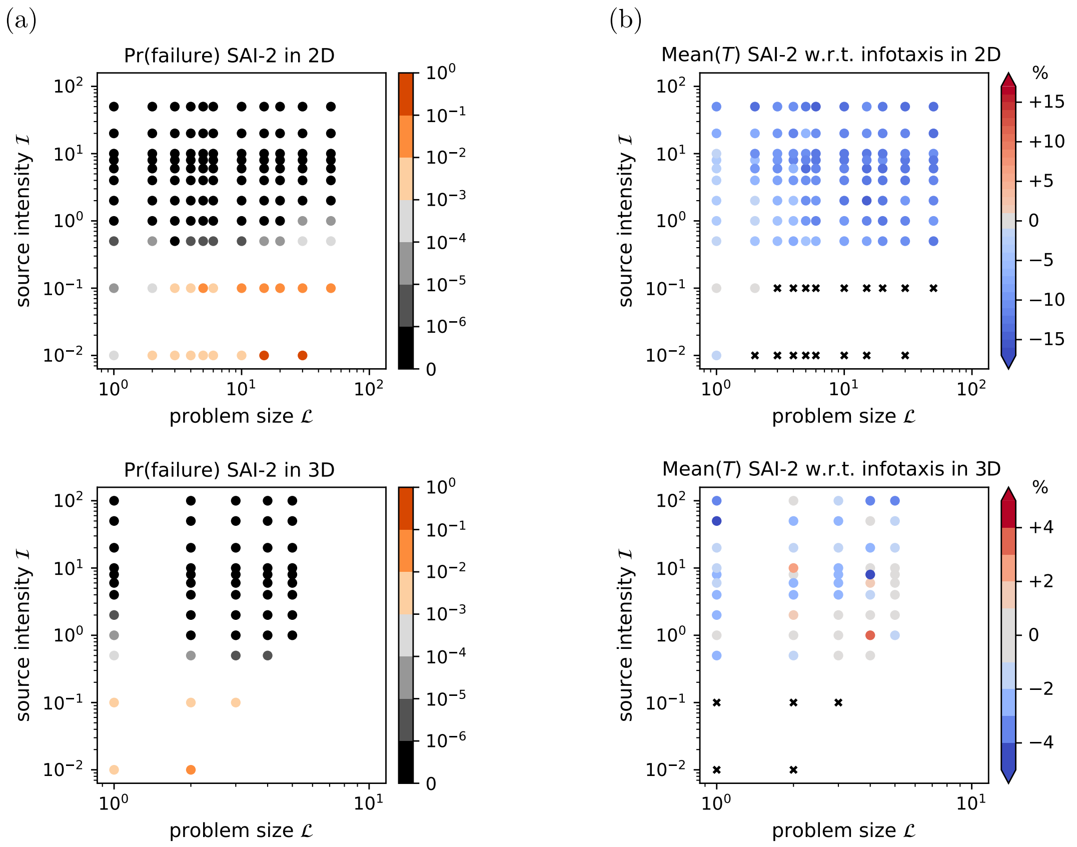


**Figure S10** Performance of space-aware infotaxis using the Euclidean norm (SAI-2) in 2D and 3D (rows), for a wide range of physical parameters $\mathcal{L}$ and $\mathcal{I}$: (a) probability of never finding the source and (b) relative difference in the mean number of steps to find the source compared to infotaxis (-10 % means that SAI finds the source in 10 % less time than infotaxis). In (b), the black crosses depict cases where Pr(failure) $> 10^{-3}$. In 1D, Manhattan and Euclidean norms are equivalent.

# 8 Additional information on deep reinforcement learning

In this section we provide additional details on our methodology for deep reinforcement learning.

## 8.1 Deep neural network

The approximate value function $\hat{v}(s; \boldsymbol{w})$ is a neural network with weights $\boldsymbol{w}$ that takes the belief state $s = [\boldsymbol{x}^a, p(\boldsymbol{x})]$ in input and returns its value (a scalar).

**Preprocessing** The belief state, which contains both the agent's position (an $n$-tuple) and the source probability distribution (an $N^n$ array, with $N$ the linear grid size and $n$ its dimensionality), is equivalently represented as a source probability distribution centered on the agent (a $(2N-1)^n$ array). This transformation, illustrated in Fig. S11, is applied to the belief state before using it as an input to the neural network.

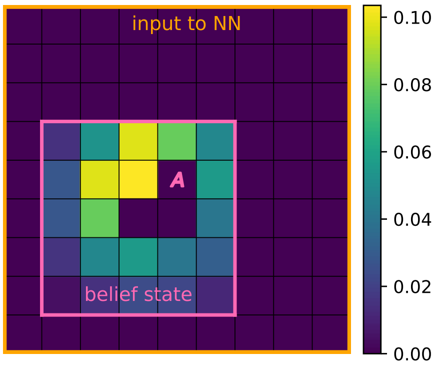


**Figure S11** Preprocessing: the belief state, which consists of the source probability distribution of size $N^n$ (pink border) and of the agent's position (depicted by a pink "A"), is transformed into a single probability distribution (orange border) of size $(2N-1)^n$ centered on the agent.

**Architecture** We use a feedforward neural network with fully connected layers: the input layer, followed by $N_{\text{hidden}}$ hidden layers with rectifier linear units (ReLU) activations, and a linear output layer. The network size (number of neurons per layer and number of hidden layers) was chosen such that more neurons does not increase performance any further. Typically we used $N_{\text{hidden}} = 3$ in most cases, with an increasing number of neurons per layer for increasing problem sizes. Note that with this type of architecture the number of weights (and the training time) does not scale well with the input size, which is why we are restricted to moderate problem sizes in 1D and 2D. For larger input sizes, a common approach is to use convolutional neural networks. The assessment of whether this alternative architecture is suitable for the source-tracking problem is left to future work.

**Initialization** Weights are initialized randomly (that is, neural networks are trained from scratch).

## 8.2 Training algorithm

The pseudo-code of our training algorithm is provided in Fig. S12.

For the loss function, we used the mean square error. We also experimented with the absolute relative error and did not find any significant difference. For exploration, we used $\epsilon$-greedy with a value of $\epsilon$ that decays exponentially during the training. The hyperparameters we used are given in Table S2. Note that these hyperparameters were not optimized (owing to the huge computational cost of such an optimization, which would have to be performed for each individual case), but chosen based on standard practice and preliminary trials. Training was performed on a single CPU with 8 cores, which leaves ample space for scaling up our approach to larger domains by parallelizing our algorithm (how to parallelize training is, however, not trivial).

Due to our choice of breaking ties arbitrarily in a deterministic manner (cf. Section 2.4), the symmetries of the agent trajectories are artificially broken (for example at the very beginning, where all actions are of equivalent value, the agent will always go east). This will introduce a bias in the belief states sampled by

```
Initialize replay memory to capacity memory_size
Initialize value function v with random weights w
Initialize target value function v⁻ with random weights w⁻ = w
converged_weights ← False
it ← 0
while not converged_weights do
                                  // Generate new experience
    epsilon ← max(epsilon_init * exp(−it/epsilon_decay), epsilon_floor)    // decaying ε of ε-greedy
    m ← 0
    episode_complete ← True
    while m < new_transitions_per_it do
        if episode_complete then
            initialize belief state s for a new episode
            episode_complete ← False
        end if
        s ← apply_random_symmetry(s)        // randomize over symmetries of the problem
        for all actions a, compute all s′ accessible from s (i.e. all outcomes (found/not found and hits))
        store (s, a, s′) in replay memory
        m ← m + 1
        with probability epsilon select a random action a,          // ε-greedy exploration
        otherwise select action a = argmin_a Σ_s′ Pr(s′|s, a)[1 + v(s′; w)]   // according to current policy
        s ← make_step_in_env (s, a)    // transition to a new belief state according to action
        episode_complete ← is_episode_complete(s)
    end while
                       // Update weights by stochastic gradient descent
    for gd_step = 1, gd_steps_per_it do
        Sample minibatch_size transitions (s, a, s′) from replay memory
        For each transition, compute targets y = min_a Σ_s′ Pr(s′|s, a)[1 + v⁻(s′; w⁻)]       // using delayed
         target network
        Perform a gradient descent step on (y − v(s; w))^2 with respect to the network parameters w
    end for

    converged_weights ← are_weights_converged()
    it ← it + 1
    every update_target_network_it iterations, reset v⁻ = v
end while
```

**Figure S12** Pseudo-code for our training algorithm.

| hyperparameter | value | description |
|---|---|---|
| learning rate | 0.001 | for stochastic gradient descent (SGD) |
| discount factor | 1.0 | no discount |
| epsilon_init | 1.0 | initial value of $\epsilon$ in $\epsilon$-greedy exploration |
| epsilon_floor | 0.1 | final value of $\epsilon$ in $\epsilon$-greedy exploration |
| epsilon_decay | [1000,10000] | time scale for decay of $\epsilon$, in number of training iterations |
| memory_size | [1000,100000] | number of transitions stored in memory |
| minibatch_size | 64 | number of transitions over which each SGD update is computed |
| new_transitions_per_it | 192 | number of transitions added to memory at each training iteration |
| gd_steps_per_it | 12 | number of SGD updates performed at each training iteration |
| update_target_network_it | 1 | frequency of target network updates, in number of training iterations |

**Table S2** List of hyperparameters (as usually defined or defined in our algorithm Fig. S12) and their values. These parameters have not been optimized, but work for all tested cases (the learned policy always converges to the near-optimal for large enough neural networks). When ranges are given, larger values are typically used for longer searches (larger domains, weaker source intensities).

the agent (symmetric states will not be sampled equally often). In this context, an original feature of our algorithm is that we restore this symmetry during training by applying, at each agent step, a random symmetry transformation to the belief state. For example, in 1D, a belief state and its mirror image (flip along the axis) are equivalent, so the belief state is flipped with a probability of 1/2. Similarly, there are 8 equivalent belief states in 2D (symmetries of the square), amongst which we choose randomly at each agent step. Informal trials suggest that this trick allows to learn faster the relevant symmetries (that is, to assign equal values to symmetric belief states). An alternative way would be to enforce symmetry constraints within the neural network. Informal trials indicate that this approach yield slower, less successful training. Similarly, enforcing concavity (a property that must be satisfied by the optimal value function) within the neural network seems to degrade training. We leave the detailed study of these interesting questions to future work.

## 8.3 Optimal (or near-optimal) policy

Training was interspersed with periodic evaluations of the current policy $\hat{\pi}$ in order to monitor its progress. After a transient, the performance reaches a plateau, which signifies that training is complete.

For each case (defined by the dimensionality of the search, $\mathcal{L}$ and $\mathcal{I}$), we repeated the training for neural networks of increasing sizes (width and depth). Beyond a certain (case-dependent) network size, performance of the learned policy stopped improving, as illustrated in Fig. S13(b). This is a good indication (though not a proof) that the learned policy is optimal or very close to optimal. In the main document, we only report the performance of such near-optimal policies. Repeated trials with different random initializations yielded identical performance, which shows the robustness of our training procedure.

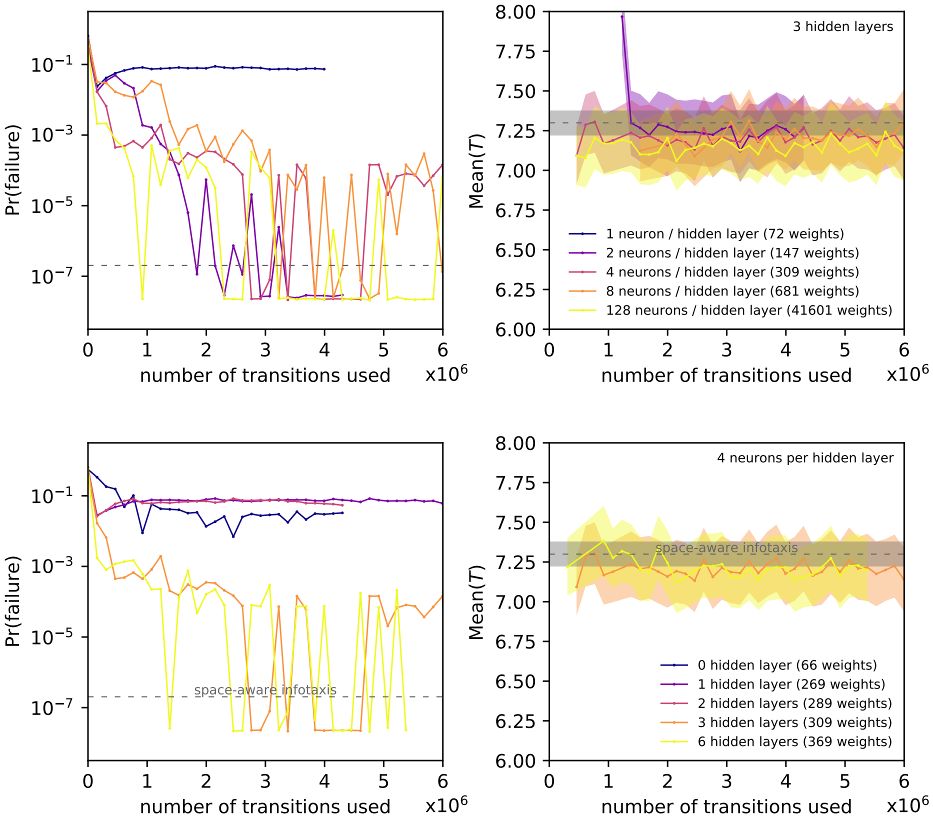


**Figure S13** Evolution of performance during training for increasing network sizes: increasing widths (top) and increasing depths (bottom). Performance is measured by Pr(failure), the probability of never finding the source (left), and by Mean($T$), the mean number of steps to reach it (right, shown only provided that Pr(failure) $< 10^{-3}$). Performance of the trained network is very reproducible over various trials, and converges to a well-defined value as the network size is increased: this defines our optimal (or near optimal) performance. Here the training was performed for a 1D search with $\mathcal{L} = 2$ and $\mathcal{I} = 2$ (grid size is $N = 33$, neural network input size is 65). The dashed lines show the performance of space-aware infotaxis. Shaded areas show 95 % confidence intervals.

# 9 List of other materials

- step-by-step illustration of how a search proceeds and how Bayesian updates are computed
- videos of the 2D and 3D searches shown in Fig. 1 of the main document
- video illustrating the hybrid Bayesian/Monte-Carlo setting
- videos of the four naive (bad) policies in 2D: greedy (x2), most likely state, voting and mean distance policies
- videos of searches with various (good) policies, with parameters summarized in Table S3

| $n$ | name | $\mathcal{L}$ | $\mathcal{I}$ | $h_{\text{init}}$ | policies |
|---|---|---|---|---|---|
| 1D | example 1 | 2 | 2 | 2 | infotaxis, SAI, RL |
| 1D | example 2 | 2 | 2 | 2 | infotaxis, SAI, RL |
| 1D | example 3 | 10 | 2 | 1 | infotaxis, SAI |
| 2D | example 1 | 1 | 2 | 1 | infotaxis, SAI, RL |
| 2D | example 2 | 2 | 2 | 1 | infotaxis, SAI, RL |
| 2D | example 3 | 5 | 2 | 1 | infotaxis, SAI |
| 2D | example 4 | 5 | 10 | 1 | infotaxis, SAI |
| 3D | example 1 | 1 | 4 | 1 | infotaxis, SAI |
| 3D | example 2 | 1 | 10 | 2 | infotaxis, SAI |

**Table S3** Parameters used in videos of searches with various (good) policies: infotaxis, space-aware infotaxis (SAI) and reinforcement learning (RL).

# References

1. Cassandra, A. R., Kaelbling, L. P. & Kurien, J. A. *Acting under Uncertainty: Discrete Bayesian Models for Mobile-Robot Navigation* in *Proceedings of IEEE/RSJ International Conference on Intelligent Robots and Systems. IROS '96* **2** (IEEE, 1996), 963–972.
2. Lochmatter, T. *Bio-Inspired and Probabilistic Algorithms for Distributed Odor Source Localization Using Mobile Robots* PhD thesis (EPFL, Lausanne, 2010).
