# Supplementary material for: Searching for a source without gradients: how good is infotaxis and how to beat it
Source: arXiv:2112.10861 ancillary file (2022-06-15)

# A step-by-step 2D search

init *p_source* (drawn from set of priors)
init *source* (drawn from *p_source*)
init *agent* (center of the domain)
$t \leftarrow 0$
*source_found* ← False
**while not** *source_found* **do**
  $t \leftarrow t + 1$
  move *agent* according to policy
  **if** *source* = *agent* **then**
    *source_found* ← True
  **else**
    *p_source*[*agent*] ← 0
    renormalize *p_source*
    compute *distance*
    compute $\mu$(*distance*)
    draw *hit* from Poisson($\mu$)
    update *p_source* using Bayes' rule
  **end**
**end**
**return** t

*t* = *0*

*source_found* = False

*p_source* =

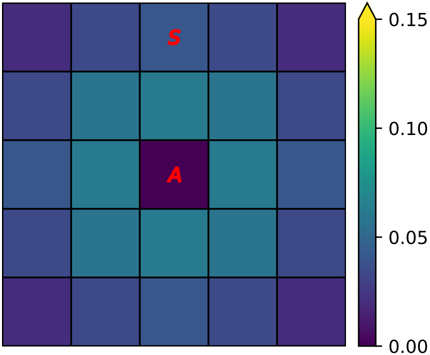

# A step-by-step 2D search

```
init p_source (drawn from set of priors)
init source (drawn from p_source)
init agent (center of the domain)
t ← 0
source_found ← False
while not source_found do
    t ← t + 1
    move agent according to policy
    if source = agent then
        source_found ← True
    else
        p_source[agent] ← 0
        renormalize p_source
        compute distance
        compute μ(distance)
        draw hit from Poisson(μ)
        update p_source using Bayes' rule
    end
end
return t
```

*t = 1*

*source_found* = False

*p_source* =

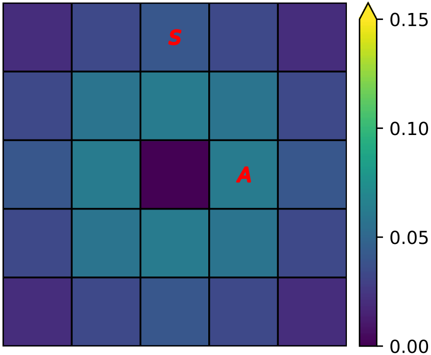

# A step-by-step 2D search

init *p_source* (drawn from set of priors)
init *source* (drawn from *p_source*)
init *agent* (center of the domain)
$t \leftarrow 0$
*source_found* ← False
**while not** *source_found* **do**
  $t \leftarrow t + 1$
  move *agent* according to policy
  **if** *source* = *agent* **then**
    *source_found* ← True
  **else**
    *p_source*[*agent*] ← 0
    renormalize *p_source*
    compute *distance*
    compute $\mu$(*distance*)
    draw *hit* from Poisson($\mu$)
    update *p_source* using Bayes' rule
  **end**
**end**
**return** t

*t* = *1*

*source_found* = False

*p_source* =

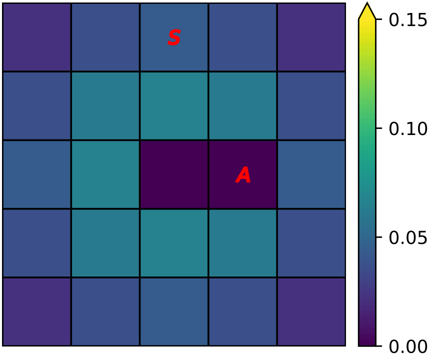

# A step-by-step 2D search

init *p_source* (drawn from set of priors)
init *source* (drawn from *p_source*)
init *agent* (center of the domain)
$t \leftarrow 0$
*source_found* ← False
**while not** *source_found* **do**
    $t \leftarrow t + 1$
    move *agent* according to policy
    **if** *source* = *agent* **then**
        *source_found* ← True
    **else**
        *p_source*[*agent*] ← 0
        renormalize *p_source*
        compute *distance*
        compute $\mu$(*distance*)
        draw *hit* from Poisson($\mu$)
        update *p_source* using Bayes' rule
    **end**
**end**
**return** t

*t = 1*

*source_found* = False

*p_source* =

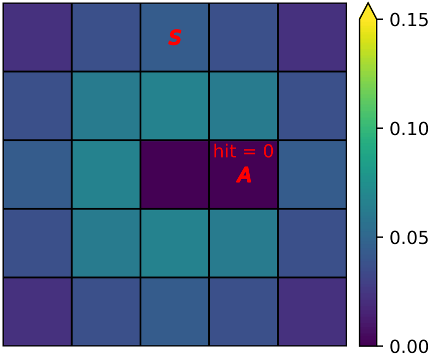

# A step-by-step 2D search

init *p_source* (drawn from set of priors)
init *source* (drawn from *p_source*)
init *agent* (center of the domain)
$t \leftarrow 0$
*source_found* ← False
**while not** *source_found* **do**
    $t \leftarrow t + 1$
    move *agent* according to policy
    **if** *source* = *agent* **then**
        *source_found* ← True
    **else**
        *p_source*[*agent*] ← 0
        renormalize *p_source*
        compute *distance*
        compute $\mu$(*distance*)
        draw *hit* from Poisson($\mu$)
        update *p_source* using Bayes' rule
    **end**
**end**
**return** t

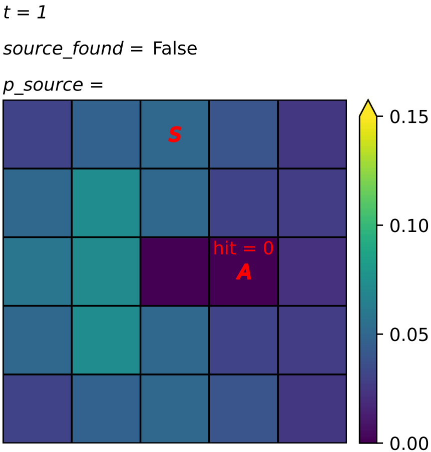

# A step-by-step 2D search

init *p_source* (drawn from set of priors)
init *source* (drawn from *p_source*)
init *agent* (center of the domain)
$t \leftarrow 0$
*source_found* $\leftarrow$ False
**while not** *source_found* **do**
    $t \leftarrow t + 1$
    move *agent* according to policy
    **if** *source* $=$ *agent* **then**
        *source_found* $\leftarrow$ True
    **else**
        *p_source*[*agent*] $\leftarrow 0$
        renormalize *p_source*
        compute *distance*
        compute $\mu$(*distance*)
        draw *hit* from Poisson($\mu$)
        update *p_source* using Bayes' rule
    **end**
**end**
**return** t

*t = 2*

*source_found* = False

*p_source* =

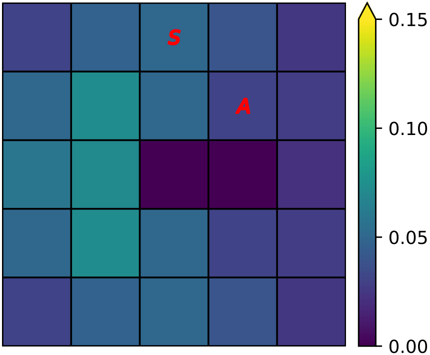

# A step-by-step 2D search

init *p_source* (drawn from set of priors)
init *source* (drawn from *p_source*)
init *agent* (center of the domain)
$t \leftarrow 0$
*source_found* ← False
**while not** *source_found* **do**
    $t \leftarrow t + 1$
    move *agent* according to policy
    **if** *source* = *agent* **then**
        *source_found* ← True
    **else**
        *p_source*[*agent*] ← 0
        renormalize *p_source*
        compute *distance*
        compute $\mu$(*distance*)
        draw *hit* from Poisson($\mu$)
        update *p_source* using Bayes' rule
    **end**
**end**
**return** t

*t* = *2*

*source_found* = False

*p_source* =

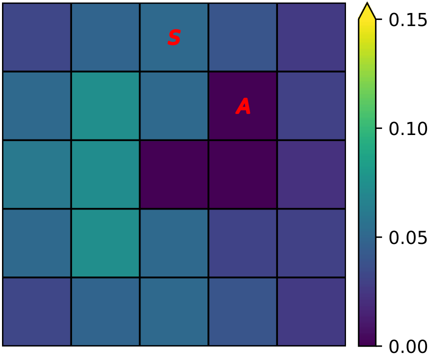

# A step-by-step 2D search

init *p_source* (drawn from set of priors)
init *source* (drawn from *p_source*)
init *agent* (center of the domain)
$t \leftarrow 0$
*source_found* ← False
**while not** *source_found* **do**
  $t \leftarrow t + 1$
  move *agent* according to policy
  **if** *source* = *agent* **then**
    *source_found* ← True
  **else**
    *p_source*[*agent*] ← 0
    renormalize *p_source*
    compute *distance*
    compute $\mu$(*distance*)
    draw *hit* from Poisson($\mu$)
    update *p_source* using Bayes' rule
  **end**
**end**
**return** t

*t* = *2*

*source_found* = False

*p_source* =

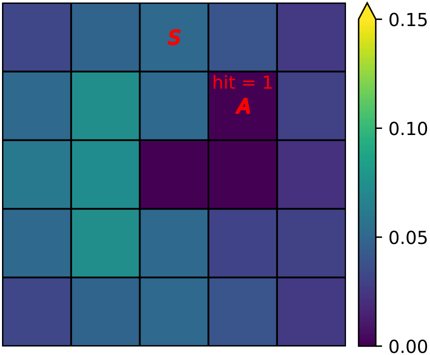

# A step-by-step 2D search

init *p_source* (drawn from set of priors)
init *source* (drawn from *p_source*)
init *agent* (center of the domain)
$t \leftarrow 0$
*source_found* ← False
**while not** *source_found* **do**
  $t \leftarrow t + 1$
  move *agent* according to policy
  **if** *source* = *agent* **then**
    *source_found* ← True
  **else**
    *p_source*[*agent*] ← 0
    renormalize *p_source*
    compute *distance*
    compute $\mu$(*distance*)
    draw *hit* from Poisson($\mu$)
    update *p_source* using Bayes' rule
  **end**
**end**
**return** t

*t* = *2*

*source_found* = False

*p_source* =

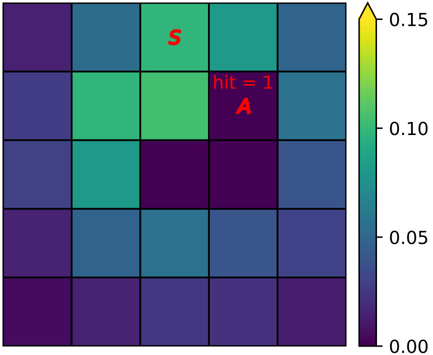

# A step-by-step 2D search

```
init p_source (drawn from set of priors)
init source (drawn from p_source)
init agent (center of the domain)
t ← 0
source_found ← False
while not source_found do
    t ← t + 1
    move agent according to policy
    if source = agent then
        source_found ← True
    else
        p_source[agent] ← 0
        renormalize p_source
        compute distance
        compute μ(distance)
        draw hit from Poisson(μ)
        update p_source using Bayes' rule
    end
end
return t
```

*t = 3*

*source_found* = False

*p_source* =

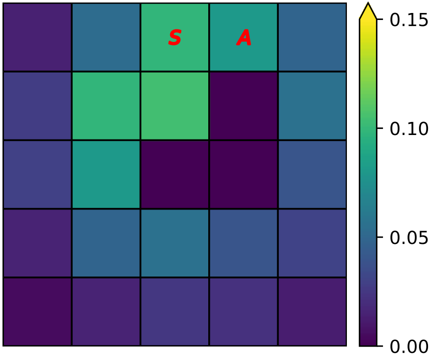

# A step-by-step 2D search

```
init p_source (drawn from set of priors)
init source (drawn from p_source)
init agent (center of the domain)
t ← 0
source_found ← False
while not source_found do
    t ← t + 1
    move agent according to policy
    if source = agent then
        source_found ← True
    else
        p_source[agent] ← 0
        renormalize p_source
        compute distance
        compute μ(distance)
        draw hit from Poisson(μ)
        update p_source using Bayes' rule
    end
end
return t
```

*t = 3*

*source_found* = False

*p_source* =

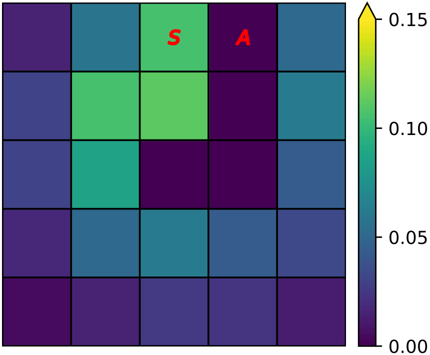

# A step-by-step 2D search

init *p_source* (drawn from set of priors)
init *source* (drawn from *p_source*)
init *agent* (center of the domain)
$t \leftarrow 0$
*source_found* ← False
**while not** *source_found* **do**
  $t \leftarrow t + 1$
  move *agent* according to policy
  **if** *source* = *agent* **then**
    *source_found* ← True
  **else**
    *p_source*[*agent*] ← 0
    renormalize *p_source*
    compute *distance*
    compute $\mu$(*distance*)
    draw *hit* from Poisson($\mu$)
    update *p_source* using Bayes' rule
  **end**
**end**
**return** t

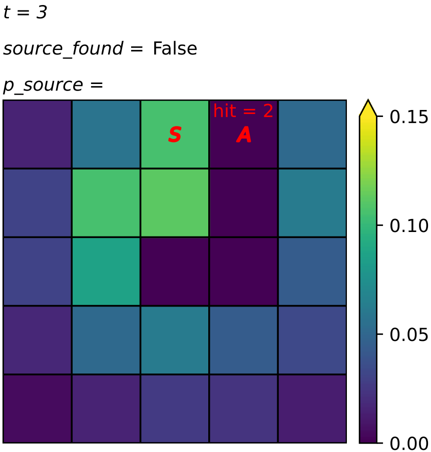

# A step-by-step 2D search

init *p_source* (drawn from set of priors)
init *source* (drawn from *p_source*)
init *agent* (center of the domain)
$t \leftarrow 0$
*source_found* ← False
**while not** *source_found* **do**
  $t \leftarrow t + 1$
  move *agent* according to policy
  **if** *source* = *agent* **then**
    *source_found* ← True
  **else**
    *p_source*[*agent*] ← 0
    renormalize *p_source*
    compute *distance*
    compute $\mu$(*distance*)
    draw *hit* from Poisson($\mu$)
    update *p_source* using Bayes' rule
  **end**
**end**
**return** t

*t* = *3*

*source_found* = False

*p_source* =

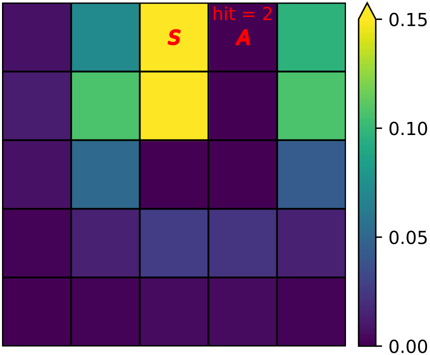

# A step-by-step 2D search

init *p_source* (drawn from set of priors)
init *source* (drawn from *p_source*)
init *agent* (center of the domain)
$t \leftarrow 0$
*source_found* $\leftarrow$ False
**while not** *source_found* **do**
  $t \leftarrow t + 1$
  move *agent* according to policy
  **if** *source* $=$ *agent* **then**
    *source_found* $\leftarrow$ True
  **else**
    *p_source*[*agent*] $\leftarrow$ 0
    renormalize *p_source*
    compute *distance*
    compute $\mu$(*distance*)
    draw *hit* from Poisson($\mu$)
    update *p_source* using Bayes' rule
  **end**
**end**
**return** t

*t = 4*

*source_found* = False

*p_source* =

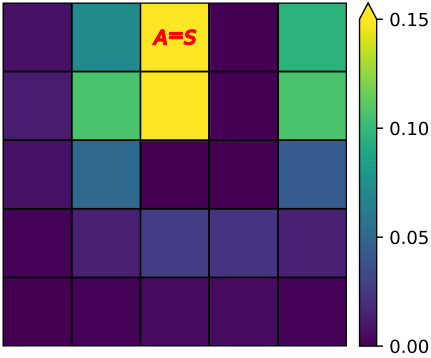

# A step-by-step 2D search

init *p_source* (drawn from set of priors)
init *source* (drawn from *p_source*)
init *agent* (center of the domain)
$t \leftarrow 0$
*source_found* ← False
**while not** *source_found* **do**
  $t \leftarrow t + 1$
  move *agent* according to policy
  **if** *source* = *agent* **then**
    *source_found* ← True
  **else**
    *p_source*[*agent*] ← 0
    renormalize *p_source*
    compute *distance*
    compute $\mu$(*distance*)
    draw *hit* from Poisson($\mu$)
    update *p_source* using Bayes' rule
  **end**
**end**
**return** t

*t* = 4

*source_found* = True

*p_source* =

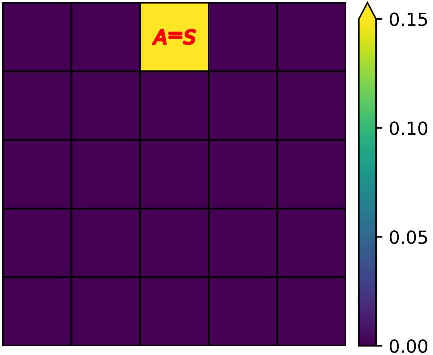

# A step-by-step 2D search

init *p_source* (drawn from set of priors)
init *source* (drawn from *p_source*)
init *agent* (center of the domain)
$t \leftarrow 0$
*source_found* ← False
**while not** *source_found* **do**
    $t \leftarrow t + 1$
    move *agent* according to policy
    **if** *source* = *agent* **then**
        *source_found* ← True
    **else**
        *p_source*[*agent*] ← 0
        renormalize *p_source*
        compute *distance*
        compute $\mu$(*distance*)
        draw *hit* from Poisson($\mu$)
        update *p_source* using Bayes' rule
    **end**
**end**
**return t**

*t = 4*

*source_found* = True

*p_source* =

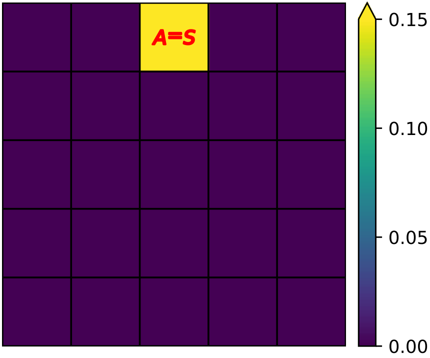

Supplement: Supplementary file 2 [file SM_example_of_step_by_step_search.pdf]
